# Supplementary material for: Self-stabilizing exchange-mediated spin transport
Source: arXiv:1811.09369 source file (2021-04-08)
Supplement: Supplementary file 1 [file supplemental.pdf]

## Supplementary Information: Self-stabilizing spin superfluid

T. Schneider,<sup>1,2,3</sup> D. Hill,<sup>4</sup> A. Kákay,<sup>1</sup> K. Lenz,<sup>1</sup> J. Lindner,<sup>1</sup> J. Fassbender,<sup>1,5</sup> P. Upadhyaya,<sup>6</sup>  
Yuxiang Liu,<sup>7</sup> Kang Wang,<sup>7</sup> Y. Tserkovnyak,<sup>4</sup> I. N. Krivorotov,<sup>8</sup> and I. Barsukov<sup>3</sup>

<sup>1</sup>*Institute of Ion Beam Physics and Materials Research,  
Helmholtz-Zentrum Dresden - Rossendorf e.V., 01328 Dresden, Germany*

<sup>2</sup>*Department of Physics, TU Chemnitz, Reichenhainer Str. 70, 09126 Chemnitz, Germany*

<sup>3</sup>*Department of Physics and Astronomy, University of California, Riverside, CA 92521, USA*

<sup>4</sup>*Department of Physics and Astronomy, University of California, Los Angeles, CA 90095, USA*

<sup>5</sup>*Institute for Physics of Solids, Technische Universität Dresden,  
Zellescher Weg 16, 01069 Dresden, Germany*

<sup>6</sup>*School of Computer and Electrical Engineering,  
Purdue University, West Lafayette, IN 47907 USA*

<sup>7</sup>*Department of Electrical and Computer Engineering,  
University of California, Los Angeles, CA 90095, USA*

<sup>8</sup>*Department of Physics and Astronomy, University of California, Irvine, CA 92697, USA*

SUPPLEMENTARY FIGURE 1: LONGITUDINAL SPIN DENSITY

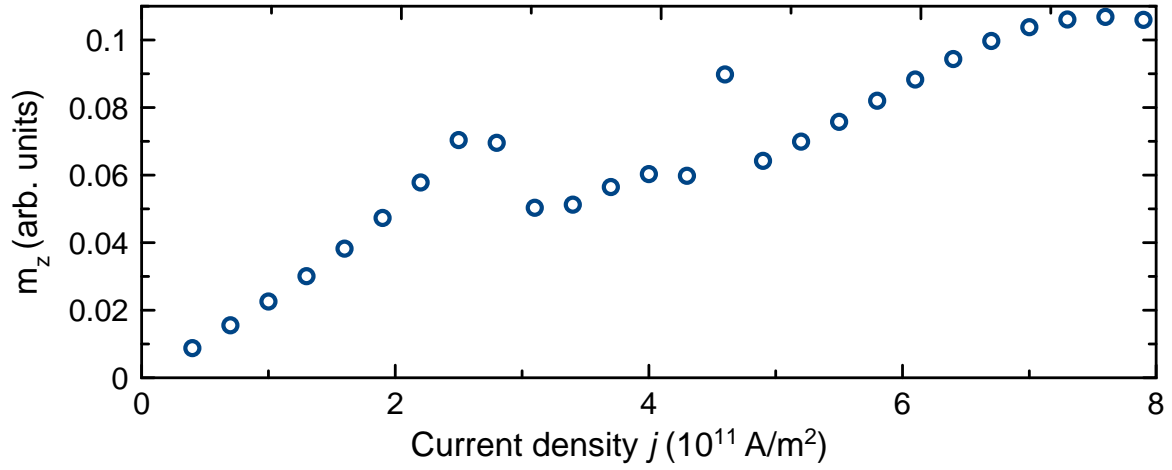

FIG. 1: Longitudinal spin density as a function of the injector current density. The values were extracted in the vicinity of the injector.

**SUPPLEMENTARY FIGURE 2: INFLUENCE OF THE INJECTOR WIDTH**

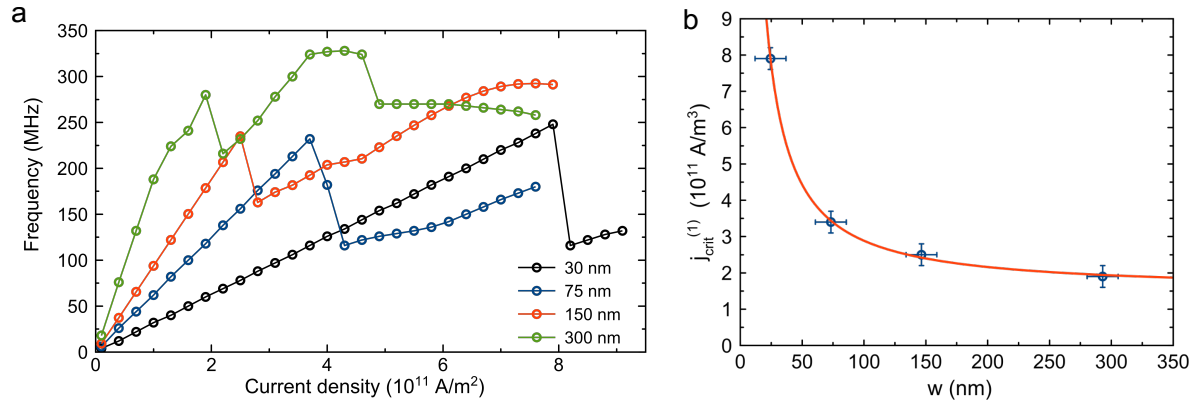

FIG. 2: Impact of the injector width on spin superfluid. (a) Base frequency  $\Omega$  for different injector widths. (b) First critical current density decreases as  $\propto 1/w$  (red line), where  $w$  is the injector width.

## SUPPLEMENTARY FIGURE 3: MAGNETIC CHARGES ALONG THE SPIN SPIRAL

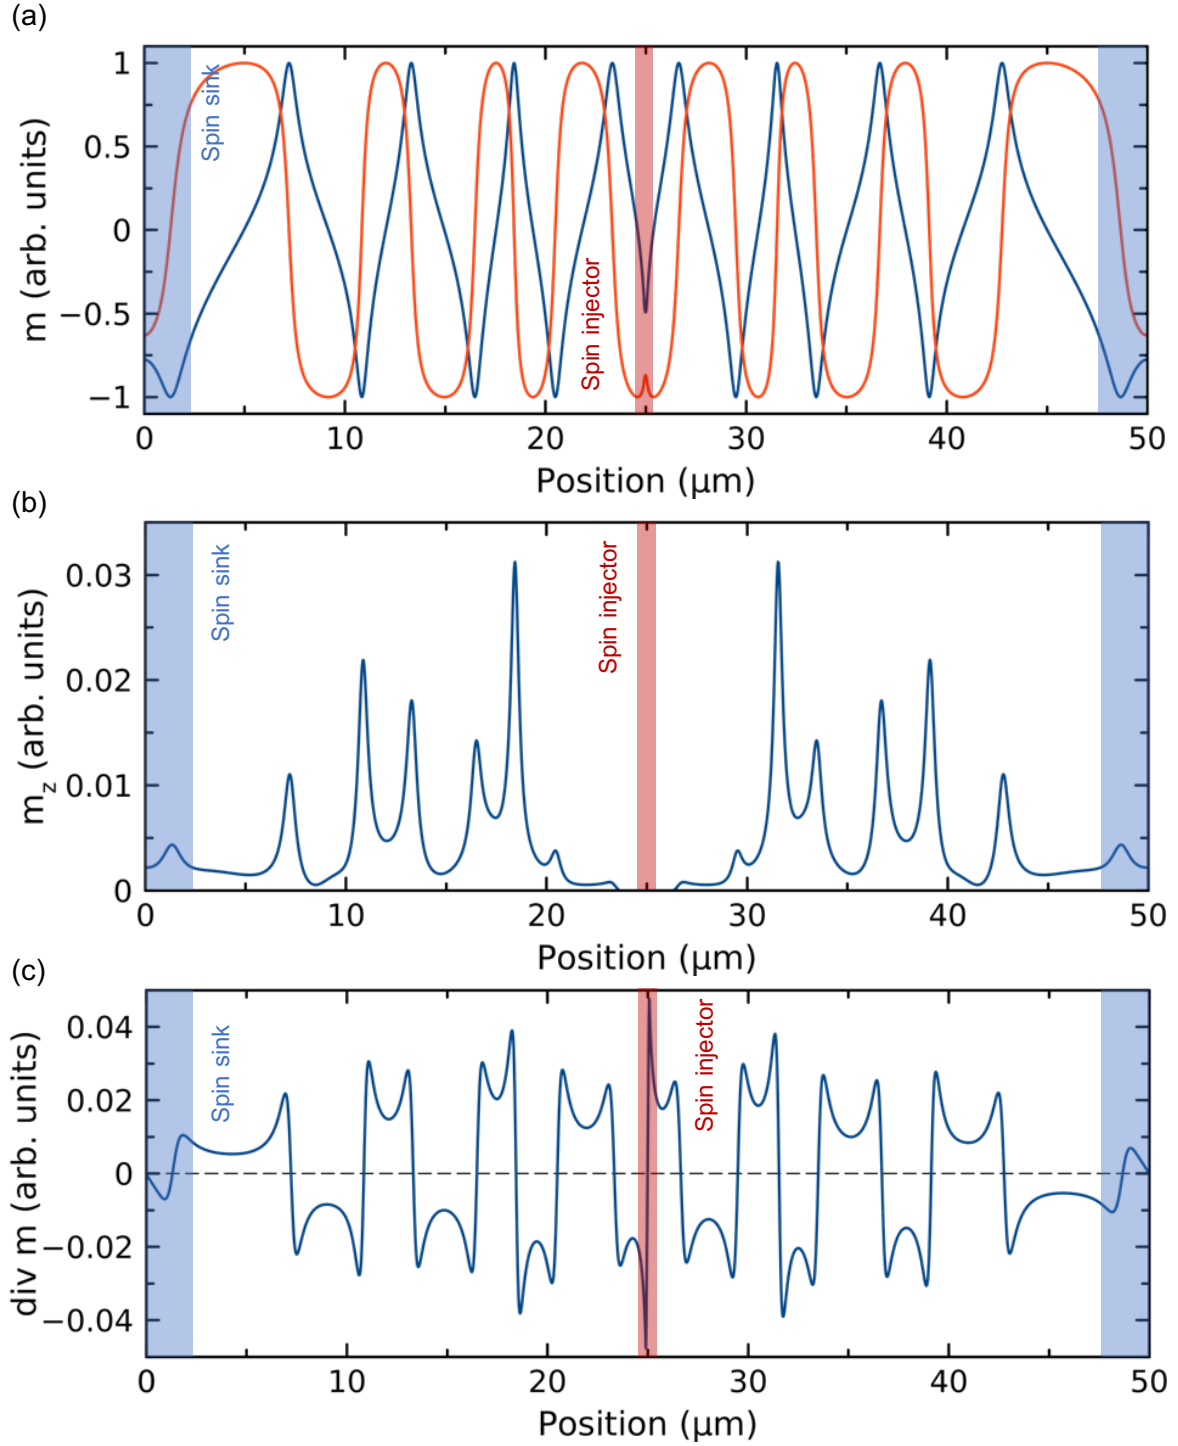

FIG. 3: Perturbations of the magnetization spiral in the presence of dipolar interaction. (a) Re-normalized in-plane components of the magnetization  $m_x$  (blue solid line) and  $m_y$  (red solid line) deviate from sinusoidal behavior. (b) Out-of-plane component  $m_z$ . The peaks in this component occur when  $m_x = -1$  and  $m_x = 1$ . (c) The divergence of the magnetization is linked to the magnetostatic field.
